# Supplementary material for: Early-Exit with Class Exclusion for Efficient Inference of Neural Networks
Source: arXiv:2309.13443 source file (2024-02-17)
Supplement: Supplementary file 1 [file appendix.tex]

\fontsize{7.0pt}{7.0}\selectfont
% \figurefontsize
 For CIFAR100, the classes from 0 to 99 are: apple, aquarium fish, baby, bear, beaver, bed, bee, beetle, bicycle, bottle, bowl, boy, bridge, bus, butterfly, camel, can, castle, caterpillar, cattle, chair, chimpanzee, clock, cloud, cockroach, couch, crab, crocodile, cup, dinosaur, dolphin, elephant, flatfish, forest, fox, girl, hamster, house, kangaroo, computer keyboard, lamp, lawn mower, leopard, lion, lizard, lobster, man, maple tree, motorbike, mountain, mouse, mushroom, oak tree, orange, orchid, otter, palm tree, pear, pickup truck, pine tree, plain, plate, poppy, porcupine, possum, rabbit, raccoon, ray, road, rocket, rose, sea, seal, shark, shrew, skunk, skyscraper, snail, snake, spider, squirrel, streetcar, sunflower, sweet pepper, table, tank, telephone, television, tiger, tractor, train, trout, tulip, turtle, wardrobe, whale, willow tree, wolf, woman, worm.
